# Supplementary material for: Principles of Lipschitz continuity in neural networks
Source: arXiv:2602.04078 source file (2026-07-10)
Supplement: Supplementary file 1 [file appendix.tex]

\subsection{Bound for Marginal Predictive Power of Frequency Features}

\begin{theorem}[Spectral Lipschitz Contribution Approximately Bounds Aumann-Shapley Value]
\label{theorem:aumann_shapley_coalition_predictive_power}
Let $S \subset \mathbb{R}^d$ be a measurable subset of frequency components, defined as a collection of frequency balls:
\begin{align}
S := \bigcup_{\zeta \in Z} B_{\delta_\zeta}(\zeta) \subset \mathbb{R}^d,
\end{align}
where $Z \subset \mathbb{R}^d$ is a set of frequency centers, and $B_{\delta_\zeta}(\zeta) := \{\omega \in \mathbb{R}^d : \|\omega - \zeta\| \leq \delta_\zeta\}$ is a frequency ball centered at frequency $\zeta \in Z$ with radius $\delta_\zeta$. 

Let $x^{(-S)}$ denote the signal obtained from $x$ by removing all frequency content in $S$. Define the characteristic function for $S$ (with respect to Lebesgue measure) as:
\begin{align}
v(S) = \Delta I_S - \inf_{S' \subseteq \mathbb{R}^d} \Delta I_{S'},
\end{align}
where $\Delta I_S = I(Q(y|x); Y) - I(Q(y|x^{(-S)}); Y)$ is the variational mutual information gap when removing frequencies in $S$. Assume $v$ is differentiable with respect to the Lebesgue measure on $\mathbb{R}^d$. For a coalition $S$ of frequency balls centered at $\zeta \in Z$, the predictive power $v(S)$, representing the contribution of $S$ to the classifier’s mutual information, satisfies:
\begin{align}
0 \leq v(S) \lesssim \int_S M_{\delta_\zeta} \cdot \varepsilon_\zeta \cdot \sqrt{\mu(B_{\delta_\zeta}(\zeta))} \, \mathrm{d}\zeta,
\end{align}
where $\varepsilon_\zeta$ is the perturbation magnitude from removing frequency ball $B_{\delta_\zeta}(\zeta)$, $\mu(B_{\delta_\zeta}(\zeta))$ is the Lebesgue measure of the frequency ball $B_{\delta_\zeta}(\zeta)$, $M_{\delta_\zeta} := \sup_{\omega \in B_{\delta_\zeta}(\zeta)} 2\pi \|\omega\| \cdot |\hat{f}(\omega)|$, and $\hat{f}$ is the Fourier transform of $f(x) = \log Q(y|x)$. 

Define the path $tS := \bigcup_{\zeta \in Z} \{\omega \in \mathbb{R}^d : \|\omega - t\zeta\| \leq t \delta_\zeta\}$, which scales the frequency balls in $S$ from the empty set ($t=0$) to the full set $S$ ($t=1$). The Aumann-Shapley value $\psi(S)$ for the coalition $S$, representing the fair allocation of predictive power among frequency components, satisfies:
\begin{align}
0 \leq \psi(S) \lesssim \int_S M_{\delta_\zeta} \cdot \varepsilon_\zeta \cdot \sqrt{\mu(B_{\delta_\zeta}(\zeta))} \, \mathrm{d}\zeta.
\end{align}
\end{theorem}

\begin{proof}

The characteristic function $v(S) = \Delta I_S - \inf_{S' \subseteq \mathbb{R}^d} \Delta I_{S'}$ is non-negative, as $\Delta I_S \geq \inf_{S' \subseteq \mathbb{R}^d} \Delta I_{S'}$, since the infimum is achieved by a set $S'$ that minimizes the mutual information gap, which can be negative or zero.

By Corollary~\ref{corollary:variational_mutual_information_bound}, for a single frequency $\zeta \in Z$, the variational mutual information gap satisfies:
\begin{align}
|\Delta I_\zeta| \lesssim M_{\delta_\zeta} \cdot \varepsilon_\zeta \cdot \sqrt{\mu(B_{\delta_\zeta}(\zeta))},
\end{align}
where $M_{\delta_\zeta} = \sup_{\omega \in B_{\delta_\zeta}(\zeta)} 2\pi \|\omega\| \cdot |\hat{f}(\omega)|$.

% Bounding the characteristic function
Since $S = \bigcup_{\zeta \in Z} B_{\delta_\zeta}(\zeta)$ is a collection of frequency balls, we assume approximate additivity of perturbations for small $\varepsilon$ over the measurable set $S$. The total mutual information gap for the coalition $S$ is approximated as:
\begin{align}
\Delta I_S \approx \int_S \Delta I_\zeta \, \mathrm{d}\zeta,
\end{align}
where the integral is over the frequency components in $S$. Thus:
\begin{align}
|\Delta I_S| \lesssim \int_S |\Delta I_\zeta| \, \mathrm{d}\zeta \lesssim \int_S M_{\delta_\zeta} \cdot \varepsilon_\zeta \cdot \sqrt{\mu(B_{\delta_\zeta}(\zeta))} \, \mathrm{d}\zeta.
\end{align}
Since $\Delta I_S \leq |\Delta I_S|$ and $\inf_{S' \subseteq \mathbb{R}^d} \Delta I_{S'} \leq 0$, we have:
\begin{align}
v(S) = \Delta I_S - \inf_{S' \subseteq \mathbb{R}^d} \Delta I_{S'} \leq |\Delta I_S| + \left|\inf_{S' \subseteq \mathbb{R}^d} \Delta I_{S'}\right|.
\end{align}
Assuming $\left|\inf_{S' \subseteq \mathbb{R}^d} \Delta I_{S'}\right| \leq |\Delta I_S|$, which holds when the infimum is achieved by a set with small or opposite-signed gap, we obtain:
\begin{align}
v(S) \lesssim \int_S M_{\delta_\zeta} \cdot \varepsilon_\zeta \cdot \sqrt{\mu(B_{\delta_\zeta}(\zeta))} \, \mathrm{d}\zeta.
\end{align}

Thus:
\begin{align}
0 \leq v(S) \lesssim \int_S M_{\delta_\zeta} \cdot \varepsilon_\zeta \cdot \sqrt{\mu(B_{\delta_\zeta}(\zeta))} \, \mathrm{d}\zeta.
\end{align}

% Deriving the approximate bound on the Aumann-Shapley value
In the Aumann-Shapley framework \citep{aumann2015values}, the Shapley value $\psi(S)$ for a coalition $S \subset \mathbb{R}^d$, defined as the collection of frequency balls $S = \bigcup_{\zeta \in Z} B_{\delta_\zeta}(\zeta)$, is given by:
\begin{align}
\psi(S) = \int_0^1 v'(t S) \, \mathrm{d} t,
\end{align}
where $tS := \bigcup_{\zeta \in Z} \{\omega \in \mathbb{R}^d : \|\omega - t\zeta\| \leq t \delta_\zeta\}$ is the path scaling the frequency balls in $S$ from the empty set ($t=0$) to the full set $S$ ($t=1$), and $v'(t S) = \frac{\mathrm{d}}{\mathrm{d} t} v(t S)$ is the directional derivative of $v$ along this path. This can be expressed as:
\begin{align}
\psi(S) = \int_S \left( \int_0^1 \frac{\partial v(t S)}{\partial \zeta} \, \mathrm{d} t \right) \mathrm{d}\zeta,
\end{align}
where $\frac{\partial v(t S)}{\partial \zeta}$ is the marginal contribution of frequency $\zeta \in S$ at scale $t$. Since $v(S)$ is non-negative and differentiable, and given the bound on $\Delta I_\zeta$:
\begin{align}
|\Delta I_\zeta| \lesssim M_{\delta_\zeta} \cdot \varepsilon_\zeta \cdot \sqrt{\mu(B_{\delta_\zeta}(\zeta))},
\end{align}
the marginal contribution $\frac{\partial v(t S)}{\partial \zeta}$ is approximately bounded by the corresponding spectral Lipschitz contribution:
\begin{align}
\frac{\partial v(t S)}{\partial \zeta} \lesssim \frac{\partial \Delta I_{t S}}{\partial \zeta} \lesssim M_{\delta_\zeta} \cdot \varepsilon_\zeta \cdot \sqrt{\mu(B_{\delta_\zeta}(\zeta))},
\end{align}
since the infimum term $\inf_{S' \subseteq \mathbb{R}^d} \Delta I_{S'}$ is constant with respect to $\zeta$ and does not contribute to the derivative. The measure of the scaled ball is $\mu(t B_{\delta_\zeta}(\zeta)) = t^d \mu(B_{\delta_\zeta}(\zeta))$, but for small $\varepsilon_\zeta$, the bound is dominated by the unscaled term $M_{\delta_\zeta} \cdot \varepsilon_\zeta \cdot \sqrt{\mu(B_{\delta_\zeta}(\zeta))}$. Integrating over $t \in [0,1]$:
\begin{align}
\int_0^1 \frac{\partial v(t S)}{\partial \zeta} \, \mathrm{d} t \lesssim M_{\delta_\zeta} \cdot \varepsilon \cdot \sqrt{\mu(B_{\delta_\zeta}(\zeta))} \cdot \int_0^1 \mathrm{d} t = M_{\delta_\zeta} \cdot \varepsilon_\zeta \cdot \sqrt{\mu(B_{\delta_\zeta}(\zeta))},
\end{align}
since $\int_0^1 \mathrm{d} t = 1$. Thus, the Aumann-Shapley value is approximately bounded as:
\begin{align}
\psi(S) = \int_S \left( \int_0^1 \frac{\partial v(t S)}{\partial \zeta} \, \mathrm{d} t \right) \mathrm{d}\zeta \lesssim \int_S M_{\delta_\zeta} \cdot \varepsilon_\zeta \cdot \sqrt{\mu(B_{\delta_\zeta}(\zeta))} \, \mathrm{d}\zeta.
\end{align}
Since $\psi(S)$ represents the total contribution of frequencies in $S$, and $v(S) \geq 0$, it follows that $\psi(S) \geq 0$. Therefore:
\begin{align}
0 \leq \psi(S) \lesssim \int_S M_{\delta_\zeta} \cdot \varepsilon_\zeta \cdot \sqrt{\mu(B_{\delta_\zeta}(\zeta))} \, \mathrm{d}\zeta.
\end{align}
This completes the proof.
\end{proof}

\begin{remark}
The theorem suggests that applying Shapley value theory in the frequency domain -- where the players correspond to frequency components -- can provide a principled way to measure the robustness of image classifiers. In this setting, the Shapley value of a frequency coalition reflects its contribution to the network’s spectral Lipschitz constant, thereby quantifying the sensitivity of the model to specific frequency bands \citep{luo2024interpreting}.
\end{remark}
