# Supplementary material for: Principles of Lipschitz continuity in neural networks
Source: arXiv:2602.04078 source file (2026-07-10)
Supplement: Supplementary file 3 [file appendix.tex]

\section{Proof: Lipschitz Constant Bounds Gradient Norm}
\label{proof:intro:lipschitz_bounds_gradient_norm}

\begin{theorem}[Lipschitz Constant Bounds Gradient Norm]
\label{theorem:gradient_lipschitz}
Let $f: \mathbb{R}^m \to \mathbb{R}$ be a differentiable function. Then $f$ is $K$-Lipschitz continuous (with respect to the 2-norm) if and only if
\begin{equation}
K = \sup_{x \in \mathrm{dom}(f)} \|\nabla f(x)\|.    
\end{equation}
\end{theorem}

\begin{proof}
\textbf{($\Rightarrow$)} Suppose $f$ is $K$-Lipschitz continuous. Then for all $x, y \in \mathbb{R}^m$,
\begin{equation}
    |f(x) - f(y)| \leq K \|x - y\|.
\end{equation}
Fix $x \in \mathbb{R}^m$ and a unit vector $v$ with $\|v\| = 1$. Define $g(t) = f(x + tv)$. Then by the chain rule,
\begin{equation}
    g'(t) = \nabla f(x + tv)^\top v,
\end{equation}
so in particular,
\begin{equation}
    |g'(0)| = |\nabla f(x)^\top v| \leq \|\nabla f(x)\|.
\end{equation}
The Lipschitz condition implies $|g(t) - g(0)| \leq K|t|$, which yields $|g'(0)| \leq K$. Since this holds for all unit vectors $v$, we have
\begin{equation}
    \|\nabla f(x)\| \leq K \quad \text{for all } x.
\end{equation}
Taking the supremum over $x$ gives
\begin{equation}
    \sup_x \|\nabla f(x)\| \leq K.
\end{equation}

\textbf{($\Leftarrow$)} Now suppose that $\|\nabla f(x)\| \leq K$ for all $x$. Let $x, y \in \mathbb{R}^m$, and define $\gamma(t) = x + t(y - x)$ for $t \in [0,1]$. Then,
\begin{equation}
    f(y) - f(x) = \int_0^1 \nabla f(\gamma(t))^\top (y - x) \, dt.
\end{equation}
By the Cauchy–Schwarz inequality,
\begin{equation}
    |f(y) - f(x)| \leq \int_0^1 \|\nabla f(\gamma(t))\| \cdot \|y - x\| \, dt \leq K \|y - x\|.
\end{equation}
Thus, $f$ is $K$-Lipschitz continuous.
\end{proof}
