# Supplementary material for: Principles of Lipschitz continuity in neural networks
Source: arXiv:2602.04078 source file (2026-07-10)
Supplement: Supplementary file 4 [file appendix.tex]

\section{Proofs: Lipschitz Constants of Activation Functions}
\label{appendix:proofs_lipschitz_constants_of_activation_functions}

\subsection{Proof: Lipschitz Constant of Sigmoid}
\label{appendix:proofs_lipschitz_constants_of_activation_functions:Sigmoid}

\begin{proof}

Consider the sigmoid function:
\begin{align}
\mathrm{Sigmoid}(x) = f(x) = (1 + e^{-x})^{-1}
.
\end{align}

Let $u = 1 + e^{-x}$, so $f(x) = u^{-1}$. The derivative is:
\begin{align}
f'(x) = -\frac{1}{u^2} \cdot \frac{du}{dx}
.
\end{align}

Compute $\frac{du}{dx}$:
\begin{align}
u = 1 + e^{-x}, \quad \frac{du}{dx} = -e^{-x}
.
\end{align}

Thus:
\begin{align}
f'(x) = -\frac{1}{(1 + e^{-x})^2} \cdot (-e^{-x}) = \frac{e^{-x}}{(1 + e^{-x})^2}
.
\end{align}

Express the derivative in terms of $f(x)$:
\begin{align}
1 - f(x) = \frac{e^{-x}}{1 + e^{-x}},
\end{align}
and:
\begin{align}
f'(x) = \frac{1}{1 + e^{-x}} \cdot \frac{e^{-x}}{1 + e^{-x}} = f(x) (1 - f(x))
.
\end{align}

Thus:

\begin{align}
|f'(x)| = f(x) (1 - f(x))
.
\end{align}

\textbf{Maximize the Derivative.} Since $0 < f(x) < 1$, we maximize $g(z) = z(1 - z)$ for $z = f(x) \in (0,1)$:
\begin{align}
g'(z) = 1 - 2z = 0 \implies z = \frac{1}{2}
,
\end{align}
thus:
\begin{align}
g\left(\frac{1}{2}\right) = \frac{1}{2} \cdot \frac{1}{2} = \frac{1}{4}
.
\end{align}

Find when $f(x) = \frac{1}{2}$:
\begin{align}
\frac{1}{1 + e^{-x}} = \frac{1}{2} \implies e^{-x} = 1 \implies x = 0
,
\end{align}
at $x = 0$:
\begin{align}
f'(0) = \frac{1}{2} \cdot \frac{1}{2} = \frac{1}{4}
.
\end{align}

As $x \to \infty$, $e^{-x} \to 0$, so $f'(x) \to 0$. As $x \to -\infty$, $e^{-x} \to \infty$, so:

\begin{align}
f'(x) \approx \frac{e^{-x}}{e^{-2x}} = e^x \to 0
.
\end{align}

Hence:
\begin{align}
    \mathrm{Lip}\left[\mathrm{Sigmoid}(x)\right] = \sup_x |f'(x)| = \frac{1}{4}.
\end{align}

\end{proof}

\subsection{Proof: Lipschitz Constant of Tanh}
\label{appendix:proofs_lipschitz_constants_of_activation_functions:Tanh}

\begin{proof}

The tanh is defined as:
\begin{align}
f(x) = \tanh(x) = \frac{e^x - e^{-x}}{e^x + e^{-x}}
,
\end{align}
for all $x, y \in \mathbb{R}$.

Let $g(x) = \sinh(x)$, $h(x) = \cosh(x)$, so $f(x) = \frac{g(x)}{h(x)}$. The derivative is:

\begin{align}
f'(x) = \frac{g'(x)h(x) - g(x)h'(x)}{h(x)^2}
.
\end{align}

Since $g'(x) = \cosh(x)$, $h'(x) = \sinh(x)$, and $h(x)^2 = \cosh^2(x)$:
\begin{align}
f'(x) = \frac{\cosh(x) \cdot \cosh(x) - \sinh(x) \cdot \sinh(x)}{\cosh^2(x)} = \frac{\cosh^2(x) - \sinh^2(x)}{\cosh^2(x)}
.
\end{align}

Using the identity $\cosh^2(x) - \sinh^2(x) = 1$:
\begin{align}
f'(x) = \frac{1}{\cosh^2(x)} = \sech^2(x).
\end{align}

Since $\cosh(x) \geq 1$, we have:
\begin{align}
|f'(x)| = \sech^2(x)    .
\end{align}

Express the derivative in terms of $f(x)$:
\begin{align}
f'(x) = \sech^2(x) = 1 - \tanh^2(x) = 1 - f(x)^2
.
\end{align}

Since $-1 \leq f(x) \leq 1$, we have $|f'(x)| = 1 - f(x)^2 \leq 1$.

\textbf{Maximize the Derivative.} Maximize $|f'(x)| = \sech^2(x)$:
\begin{align}
\cosh(x) = \frac{e^x + e^{-x}}{2}
.
\end{align}

At $x = 0$:
\begin{align}
\cosh(0) = \frac{e^0 + e^0}{2} = 1, \quad \sech^2(0) = \frac{1}{\cosh^2(0)} = 1
.
\end{align}

As $|x| \to \infty$, $\cosh(x) \approx \frac{e^{|x|}}{2}$, so:
\begin{align}
\sech^2(x) \approx \frac{4}{e^{2|x|}} \to 0
.
\end{align}

The supremum of $|f'(x)|$ is 1 at $x = 0$. Alternatively, since $f(x)^2 \leq 1$, the supremum of $1 - f(x)^2$ occurs when $f(x) = 0$:
\begin{align}
\tanh(0) = 0, \quad f'(0) = 1 - 0^2 = 1
.
\end{align}

Hence:
\begin{align}
    \mathrm{Lip}\left[\tanh(x)\right] = \sup_x |f'(x)| = 1.
\end{align}

\end{proof}

\subsection{Proof: Lipschitz Constant of Softplus}
\label{appendix:proofs_lipschitz_constants_of_activation_functions:Softplus}

\begin{proof}

Consider the softplus function:
\begin{align}
f(x) = \ln(1 + e^x)
.
\end{align}

The derivative is:
\begin{align}
f'(x) = \frac{d}{dx} \ln(1 + e^x) = \frac{e^x}{1 + e^x}
.
\end{align}

Since $e^x > 0$ and $1 + e^x > 1$, we have $f'(x) > 0$, so:
\begin{align}
|f'(x)| = \frac{e^x}{1 + e^x}
.
\end{align}

\textbf{Maximize the Derivative.} To find the Lipschitz constant, we need to compute:
\begin{align}
K = \sup_{x \in \mathbb{R}} \frac{e^x}{1 + e^x}.
\end{align}

Notice that $\frac{e^x}{1 + e^x}$ is the sigmoid function, which ranges between 0 and 1. Analyze its behavior:
\begin{enumerate}
    \item As $x \to \infty$, $e^x$ grows large, so:
    \begin{align}
    \frac{e^x}{1 + e^x} \approx \frac{e^x}{e^x} = 1
    .
    \end{align}

    \item As $x \to -\infty$, $e^x \to 0$, so:
    \begin{align}
    \frac{e^x}{1 + e^x} \to \frac{0}{1} = 0.
    \end{align}

\end{enumerate}

To confirm the supremum, consider the function $g(x) = \frac{e^x}{1 + e^x}$. Its derivative is:
\begin{align}
g'(x) = \frac{e^x (1 + e^x) - e^x \cdot e^x}{(1 + e^x)^2} = \frac{e^x}{(1 + e^x)^2}
.
\end{align}

Since $g'(x) > 0$ for all $x$, $g(x)$ is strictly increasing, approaching 0 as $x \to -\infty$ and 1 as $x \to \infty$. Thus:
\begin{align}
\sup_{x \in \mathbb{R}} \frac{e^x}{1 + e^x} = 1
\end{align}

Hence:
\begin{align}
    \mathrm{Lip}\left[\mathrm{Softplus}(x)\right] = \sup_x |f'(x)| = 1.
\end{align}

\end{proof}

\subsection{Proof: Lipschitz Constant of Swish}
\label{appendix:proofs_lipschitz_constants_of_activation_functions:Swish}
\begin{proof}
Let
\begin{align}
f(x) = x\,\sigma(x), \quad \sigma(x) = \frac{1}{1+e^{-x}}.
\end{align}
The derivative is
\begin{align}
g(x) := f'(x) = \sigma(x) + x\,\sigma(x)\bigl(1 - \sigma(x)\bigr).
\end{align}
Since $\sigma(-x) = 1 - \sigma(x)$, we have
\begin{align}\label{eq:sym}
g(-x) = 1 - g(x)
.
\end{align}

% Set:
% \begin{align}
%    K: = \sup_x |g(x)|. 
% \end{align}

Using $\sigma(x) = \frac12\bigl(1 + \tanh(\frac{x}{2})\bigr)$ and $\sigma(x)(1-\sigma(x)) = \frac14\operatorname{sech}^2(\frac{x}{2})$,
\begin{align}
g(x) = \frac12\Bigl(1 + \tanh\!\frac{x}{2}\Bigr) + \frac{x}{4}\,\operatorname{sech}^2\!\frac{x}{2}.
\end{align}
Differentiating,
\begin{align}
g'(x) = \frac14\,\operatorname{sech}^2\!\frac{x}{2} \,\Bigl( 2 - x\,\tanh\!\frac{x}{2} \Bigr),
\end{align}
so the maximizer $x^\star>0$ satisfies
\begin{align}
x^\star\,\tanh\!\frac{x^\star}{2} = 2.
\end{align}

Using $\tanh(\frac{x^\star}{2}) = \frac{2}{x^\star}$ and
\begin{align}
\operatorname{sech}^2\!\frac{x^\star}{2} = \frac{(x^\star)^2 - 4}{(x^\star)^2}.
\end{align}

Thus
\begin{align}
K = g(x^\star)
= \frac12 + \frac{x^\star}{4}.
\end{align}

Since $g(-x) = 1 - g(x)$, $x^\star$ gives the global maximum of $|g|$, solving $x^\star\,\tanh\!\frac{x^\star}{2} = 2$ gives:
\begin{align}
x^\star \approx 2.3993572805\cdots
.
\end{align}

Hence:
\begin{align}
    \mathrm{Lip}\left[\mathrm{Siwsh}(x)\right] = \sup_x |f'(x)| \approx 1.09983932\cdots
\end{align}

\end{proof}

\subsection{Proof: Lipschitz constant of GELU}
\label{appendix:proofs_lipschitz_constants_of_activation_functions:GELU}
\begin{proof}

Let:
\begin{align}
f(x) = x\,\Phi(x),
\end{align}
where: 
\begin{align}
\Phi(x) = \tfrac12\bigl(1+\operatorname{erf}(x/\sqrt{2})\bigr)  
\end{align}
is the standard normal CDF and: 
\begin{align}
\phi(x)=\tfrac{1}{\sqrt{2\pi}}e^{-x^2/2}    
\end{align}
is its PDF. 

Differentiate:
\begin{align}
g(x):=f'(x)=\Phi(x)+x\,\phi(x).
\end{align}

Note the symmetry $\Phi(-x)=1-\Phi(x)$ and $\phi(-x)=\phi(x)$, hence
\begin{align}
g(-x)=1-g(x).
\end{align}

Compute the critical points:
\begin{align}
g'(x)=\phi(x)+\phi(x)+x\,\phi'(x)
      =2\phi(x) - x^2\phi(x)
      =\phi(x)\,(2-x^2).
\end{align}

Since $\phi(x)>0$, we have $g'(x)>0$ for $|x|<\sqrt{2}$ and $g'(x)<0$ for $|x|>\sqrt{2}$. Hence $g$ attains its unique global maximum at $x^\star=\sqrt{2}$ and minimum at $-\sqrt{2}$. 

Since $g(-x)=1-g(x)$, the minimum equals $1-g(\sqrt{2})$, so indeed $\sup_x|g(x)|=g(\sqrt{2})$.

Evaluate at:
\begin{align}
x=\sqrt{2} \approx 1.414224\cdots    
,
\end{align}
hence:
\begin{align}
\mathrm{Lip}\left[\mathrm{GELU}(x)\right] &= \sup_x |f'(x)| \\
&= g(\sqrt{2}) \\
&= \Phi(\sqrt{2})+\sqrt{2}\,\phi(\sqrt{2}) \\
&= \tfrac12\bigl(1+\operatorname{erf}(1)\bigr) + \frac{e^{-1}}{\sqrt{\pi}} \\
&\approx 1.128904145
.
\end{align}

\end{proof}

\subsection{Proof: Lipschitz constant of Softmax}
\label{appendix:proofs_lipschitz_constants_of_activation_functions:Softmax}

\begin{proof}
Let
\begin{align}
\operatorname{softmax}(z)_i=\frac{e^{z_i}}{\sum_{j=1}^n e^{z_j}}
,
\end{align}
and:
\begin{align}
p:=\operatorname{softmax}(z)\in \Delta^{n-1}
,
\end{align}
where $\Delta^{n-1}$ is the probability simplex in $\mathbb{R}^n$ (\ie, the set of all probability vectors of length $n$):
\begin{align}
\Delta^{n-1} \;:=\; \big\{\, p \in \mathbb{R}^n \ \big|\ p_i \ge 0,\ \sum_{i=1}^n p_i = 1 \,\big\}.
\end{align}

The Jacobian is
\begin{align}
J(z)=\nabla \operatorname{softmax}(z)=\mathrm{diag}(p)-p\,p^\top,
\end{align}
which is symmetric positive semidefinite (PSD) and satisfies:
\begin{align}
J(z)\,\mathbf{1}=0.    
\end{align}

Hence the Lipschitz constant $K$ is:
\begin{align}
K=\sup_{z\in\mathbb{R}^n}\|J(z)\|_2=\sup_{p\in\Delta^{n-1}}\lambda_{\max}\!\big(\mathrm{diag}(p)-p\,p^\top\big).
\end{align}
where $\lambda_{\max}$ is the largest singular value of $\mathrm{diag}(p)-p\,p^\top$.

For any unit vector $v\in\mathbb{R}^n$,
\begin{align}
v^\top J(z)\,v
= v^\top\!\mathrm{diag}(p)\,v - (p^\top v)^2
= \sum_{i=1}^n p_i v_i^2 - \Big(\sum_{i=1}^n p_i v_i\Big)^2
= \mathrm{Var}_{i\sim p}[v_i].
\end{align}

Therefore
\begin{align}
\|J(z)\|_2=\sup_{\|v\|_2=1}\mathrm{Var}_{i\sim p}[v_i].
\end{align}

By Popoviciu’s inequality on variances, for any random variable $X$ supported in $[a,b]$,
\begin{align}
\mathrm{Var}[X]\le \frac{(b-a)^2}{4},
\end{align}
with equality attained by a two–point distribution at the endpoints. 

Applying this to $X=v_i$ under $p$, we get
\begin{align}
\mathrm{Var}_{i\sim p}[v_i] \le \frac{\big(\max_i v_i-\min_i v_i\big)^2}{4}.
\end{align}

% To bound the right-hand side for $\|v\|_2 = 1$, note that
% \begin{align}
% \max_i v_i - \min_i v_i \le \sqrt{ (1)^2 + (1)^2 } = \sqrt{2},
% \end{align}
% because the largest possible spread occurs when $v$ has only two distinct values, one positive and one negative, each appearing in exactly one coordinate, with all other coordinates zero.  
% For $\|v\|_2 = 1$, the optimal choice is
% \begin{align}
% v = \frac{1}{\sqrt{2}} (e_a - e_b),
% \end{align}
% where $e_a, e_b$ are standard basis vectors for distinct indices $a \neq b$.  
% In this case $\max_i v_i = 1/\sqrt{2}$ and $\min_i v_i = -1/\sqrt{2}$, so $\max_i v_i - \min_i v_i = \sqrt{2}$.

% Therefore,
% \begin{align}
% \sup_{\|v\|_2 = 1} \operatorname{Var}_{i\sim p}(v_i)
% \le \frac{(\sqrt{2})^2}{4} = \frac12,
% \end{align}
% and equality is approached when $p$ is supported equally on the two coordinates $a$ and $b$.

Maximizing the RHS over $\|v\|_2=1$ yields $\max_i v_i-\min_i v_i\le \sqrt{2}$, with equality for
\begin{align}
v=\frac{1}{\sqrt{2}}(e_a-e_b)\quad\text{for some distinct }a,b,
\end{align}
so that
\begin{align}
\sup_{\|v\|_2=1}\mathrm{Var}_{i\sim p}[v_i]
\le 
\frac{(\sqrt{2})^2}{4}=\frac12.
\end{align}

This upper bound is (arbitrarily) attainable by choosing $p$ supported on the two indices $a,b$ with $p_a=p_b=\tfrac12$ and $p_i\to 0$ for $i\notin\{a,b\}$ (which is approached by softmax logits $z_a=z_b\gg z_{i\notin\{a,b\}}$). In that case,
\begin{align}
J=\begin{bmatrix}
\frac14 & -\frac14 \\[2pt] -\frac14 & \frac14
\end{bmatrix}\oplus 0_{n-2},
\end{align}
whose largest eigenvalue is $\tfrac12$.

Hence:
\begin{align}
    \mathrm{Lip}\left[\mathrm{Softmax}(x)\right] = \sup_z \|J(z)\|_2 = \frac{1}{2},
\end{align}
independent of $n\ge 2$. %For comparison, at the uniform point $p_i=\tfrac1n$ one has $J=\tfrac1n I-\tfrac{1}{n^2}\mathbf{1}\mathbf{1}^\top$ with $\|J\|_2=\tfrac1n\le \tfrac12$, consistent with the global maximum.

\end{proof}
