# Supplementary material for: Principles of Lipschitz continuity in neural networks
Source: arXiv:2602.04078 source file (2026-07-10)
Supplement: Supplementary file 7 [file appendix.tex]

\section{Notes}
We derive the first-order and the second-order derivatives of singular value function without using perturbation theory for linear operators.

\section{Setting}

Let $A \in \mathbb{R}^{m \times n}$ admit a singular value decomposition (SVD):
\begin{align}
A = U \Sigma V^\top    
\end{align}
where:
\begin{align}
    U = (u_1, u_2, \dots, u_m) \in \mathbb{R}^{m \times m}
\end{align}
and:
\begin{align}
    \Sigma = \operatorname{diag}(\sigma_1, \sigma_2, \dots, \sigma_r, 0, \dots, 0) \in \mathbb{R}^{m \times n} 
\end{align}
and:
\begin{align}
    \sigma_1 \geq \sigma_2 \geq \dots \geq \sigma_r > 0
\end{align}
and:
\begin{align}
    V = (v_1, v_2, \dots, v_n).
\end{align}

\begin{property}
Following properties hold:
\begin{align}
        A = \sigma_1 u_1 v_1^\top + \sigma_2 u_2 v_2^\top + \cdots + \sigma_r u_r v_r^\top 
\end{align}
and:
\begin{align}
    u_i^\top A = \sigma_i v_i^\top 
\end{align}
and:
\begin{align}
    A^\top u_i = \sigma_i v_i
\end{align}
and:
\begin{align}
    A v_i = \sigma_i u_i.
\end{align}
\end{property}

\begin{definition}[Singular value function]
Let $\sigma_k: \mathbb{R}^{m \times n} \mapsto \mathbb{R}_{+}$ be the singular value function. The $k$-th largest singular value of matrix $A$ is given by $\sigma_k(A)$.  
\end{definition}

\section{First-Order Derivative}
\begin{lemma}
The identity regarding the total derivative $df$ and the derivative $\frac{\partial f}{\partial X}$ holds:
\begin{align}
    df &= \sum_{i=1}^m \sum_{j=1}^{n} \left[\frac{\partial f}{\partial X}\right]_{i,j} \left[dX \right]_{i,j} \\
    &= \sum_{i=1}^m \sum_{j=1}^{n} \left[ \frac{\partial f}{\partial X} \odot dX\right]_{i,j} \\
    &= \left\langle \frac{\partial f}{\partial X}, dX \right\rangle \\
    &= \operatorname{Tr}\left( \left(\frac{\partial f}{\partial X}\right)^\top dX \right)
\end{align}
where $\left[\cdot\right]_{i,j}$ denotes the element of $\cdot$ at $i,j$. We have used the identity:
\begin{align}
\left\langle A, B \right\rangle  = \operatorname{Tr}\left( A^\top B \right).
\end{align}
\label{lemma:first_order_derivative_identity}
\end{lemma}

\begin{lemma}
    The following identity holds:
        \begin{align}
            \sigma_k = u_k^\top A v_k.
        \end{align}
        \label{lemma:singular_value_identity}
\end{lemma}

\begin{proof}
    Since:
    \begin{align}
        A = \sigma_1 u_1 v_1^\top + \cdots + \sigma_k u_k v_k^\top + \cdots + \sigma_r u_r v_r^\top. 
    \end{align}
Left multiply by $u_k^\top$:
\begin{align}
 u_k^\top A &= u_k^\top (\sigma_1 u_1 v_1^\top + \cdots + \sigma_k u_k v_k^\top + \cdots + \sigma_r u_r v_r^\top) \\
 &= \sigma_k v_k^\top.
\end{align}
Right multiply by $v_k^\top$:
\begin{align}
   u_k^\top A v_k = \sigma_k. 
\end{align}
\end{proof}

\begin{lemma}[Total Derivative of $\sigma_k$]
\label{lemma:total_derivative_simga_k}
Using Lemma~\ref{lemma:singular_value_identity}, the total derivative of $\sigma_k$ is given as:
\begin{align}
    d \sigma_k = du_k^\top A v_k + u_k^\top dA v_k + u_k^\top A dv_k.
\end{align}    
The perturbations on singular value functions are independent to left and right singular value vectors. Thus:
\begin{align}
    d \sigma_k = u_k^\top dA v_k.
\end{align}
\end{lemma}

\begin{theorem}[First-Order Derivative of $\sigma_k$]
    \begin{align}
        \frac{\partial \sigma_k}{dA} = u_k v_k.
    \end{align}
    \label{theo:jacobian_sigma_k}
\end{theorem}

\section{Second-Order Derivative}

    \begin{property}
The following properties will help us to derive the Hessian:
\begin{align}
\operatorname{vec}\left(AXB\right) = (B^\top \otimes A)  \operatorname{vec}\left(X\right)       
\end{align}
and:
\begin{align}
    \operatorname{vec}\left(ab^\top\right) = b \otimes a
\end{align}
and:
\begin{align}
    (A \otimes B)(C \otimes D) = (AC) \otimes (BD)
\end{align}
where $\otimes$ denotes Kronecker product.
\end{property}

\subsection{Representing total derivatives with complete bases}
We aim to derive $du_k$ and $dv_k$. Consider the total derivative for:
\begin{align}
    d\sigma_k = u_kv_k.
\end{align}

Since:
\begin{align}
    Av_k = \sigma_k u_k
\end{align}
and:
\begin{align}
    A^\top u_k = \sigma_k v_k.
\end{align}

Consider total derivatives:
\begin{align}
    d(Av_k) = d (\sigma_k u_k) \\
    \Longrightarrow dA v_k + A dv_k = d\sigma_k u_k + \sigma_k du_k
\end{align}
and:
\begin{align}
    d(A^\top u_k) = d(\sigma_k v_k) \\
    \Longrightarrow dA^\top u_k + A^\top du_k = d\sigma_k v_k + \sigma_k dv_k.
\end{align}

We have an equation system:
\begin{align}
\begin{cases}
dA v_k + A dv_k = d\sigma_k u_k + \sigma_k du_k \\
dA^\top u_k + A^\top du_k = d\sigma_k v_k + \sigma_k dv_k
\end{cases}.
\end{align}

\begin{definition}
To fully capture $d u_k$ and $v_k$, we expand them using complete orthonormal bases of $U$ and $V$:
\begin{align}
    \begin{cases}
    du_k = \sum_{i=1}^{m} a_{k, i} u_i  &i \neq k \\
    dv_k = \sum_{j=1}^{n} b_{k, j} v_j  &j \neq k
    \end{cases}.
\end{align}
We exclude the bases $u_k$ and $v_k$ because there are no contributions on them:
\begin{align}
    \textcolor{red}{d (u_k^\top u_k) = d (1) \Longrightarrow d u_k = 0}
\end{align}
and:
\begin{align}
    \textcolor{red}{d (v_k^\top v_k) = d (1) \Longrightarrow d v_k = 0}.
\end{align}
    \end{definition}

\subsection{Solving $a_{k,i}$ and $b_{k, j}$}

    Left-multiply:
\begin{align}
 dA v_k + A dv_k = d\sigma_k u_k + \sigma_k du_k   
\end{align}
by $u_i^\top $:
\begin{align}
    &u_i^\top(dA v_k + A dv_k) = u_i^\top(d\sigma_k u_k + \sigma_k du_k) \\
    &\Longrightarrow u_i^\top dA v_k + u_i^\top A dv_k = u_i^\top d\sigma_k u_k + u_i^\top \sigma_k du_k .
\end{align}

For $i \neq k$ and $i \leq r$:
\begin{align}
    &u_i^\top dA v_k + u_i^\top A dv_k = u_i^\top d\sigma_k u_k + u_i^\top \sigma_k du_k \\
    &\Longrightarrow u_i^\top dA v_k + u_i^\top A dv_k = u_i^\top \sigma_k du_k.
\end{align}

Using the result:
\begin{align}
    u_i^\top A = \sigma_i v_i^\top 
\end{align}
and:
\begin{align}
u_i^\top  du_k =    u_i^\top \sum_{j \neq k} a_{k,j}u_j = a_{k,i} 
\end{align}
and:
\begin{align}
    v_i^\top  dv_k =    v_i^\top \sum_{j \neq k} b_{k,j}v_j = b_{k,i} .
\end{align}

Hence:
\begin{align}
  &u_i^\top dA v_k + \textcolor{red}{u_i^\top A dv_k} = \textcolor{red}{u_i^\top \sigma_k du_k} \\
  &\Longrightarrow \textcolor{red}{\sigma_i v_i^\top dv_k} + u_i^\top dA v_k = \textcolor{red}{\sigma_k a_{k, i}} \\
  &\Longrightarrow \textcolor{red}{\sigma_i b_{k,i}} + s_{i,k} = \textcolor{red}{\sigma_k a_{k, i}} 
\end{align}
where:
\begin{align}
    s_{i,k} = u_i^\top dA v_k.
\end{align}

Left-multiply:
\begin{align}
    dA^\top u_k + A^\top du_k = d\sigma_k v_k + \sigma_k dv_k
\end{align}
by $v_i^\top$ :
\begin{align}
    &v_i^\top(dA^\top u_k + A^\top du_k) = v_i^\top(d\sigma_k v_k + \sigma_k dv_k) \\
    &\Longrightarrow v_i^\top dA^\top u_k + v_i^\top A^\top du_k = v_i^\top d\sigma_k v_k + v_i^\top \sigma_k dv_k 
\end{align}

For $i \neq k$, using:
\begin{align}
    v_i^\top A^\top = \sigma_i u_i^\top
\end{align}
and:
\begin{align}
    u_i^\top du_k = a_{k,i}
\end{align}
and:
\begin{align}
    v_i^\top v_k = b_{k, i}
\end{align}
and:
\begin{align}
    s_{k, i} = u_k^\top dA v_i.
\end{align}
We have:
\begin{align}
    & v_i^\top dA^\top u_k + \textcolor{red}{v_i^\top A^\top du_k }= v_i^\top d\sigma_k v_k + \textcolor{red}{v_i^\top \sigma_k dv_k } \\
    &\Longrightarrow s_{k, i} + \textcolor{red}{\sigma_iu_i^\top du_k} = \sigma_k b_{k,i}
\end{align}

\section{Solving for $a_{k,i}$ and $b_{k,i}$}

We form the system of equations for $i = 2, \dots, rank(A)$:
\begin{align}
    \begin{cases}
    \sigma_k a_{k,i} - \sigma_i b_{k,i} &= s_{i,k} \\
- \sigma_i a_{k,i} + \sigma_k b_{k,i} &= s_{k,i}
    \end{cases}.
\end{align}

Set:
\begin{align}
    M = \begin{pmatrix} 
        \sigma_k  & -\sigma_i \\ 
        -\sigma_i & \sigma_k \end{pmatrix}.
\end{align}

Then:
\begin{align}
M
\begin{pmatrix}
a_{k,i} \\
b_{k,i}
\end{pmatrix}
\begin{pmatrix}
s_{i,k} \\
s_{k,i}
\end{pmatrix}
\end{align}

Thus:
\begin{align}
\det(M) = \sigma_k^2 - \sigma_i^2. 
\end{align}

\subsection{Case 1: $\sigma_i \ne 0$ for $i \leq r$ and $i \neq k$}

Since the determinant $\sigma_k^2 - \sigma_i^2 \neq 0$, we solve:
\begin{align}
\begin{cases}
a_{k,i} &= \frac{\sigma_k s_{i,k} + \sigma_i s_{k,i}}{\sigma_k^2 - \sigma_i^2} \\
b_{k,i} &= \frac{\sigma_i s_{i,k} + \sigma_k s_{k,i}}{\sigma_k^2 - \sigma_i^2}.
\end{cases}
\end{align}

\subsection{Case 2: $\sigma_i = 0$ for $j > r$}

The equations simplify to:
\begin{align}
\begin{cases}
a_{k,i} &= \frac{s_{i,k}}{\sigma_k} \\
b_{k,i} &= \frac{s_{k,i}}{\sigma_k}.
\end{cases}
\end{align}

\section{Total derivative of $d\sigma_k$}

The total derivative of $d\sigma_k$:
\begin{align}
    d^2\sigma_k =  \sum_{i \neq k} \left( a_{k,i} s_{i,k} + b_{k,i} s_{k,i} \right).
\end{align}

\subsection{Case 1: $\sigma_i \ne 0$}

\begin{align}
    d^2\sigma_k|_{\sigma_i \neq 0} = \sum_{i \neq k, i=1}^{r} \frac{\sigma_k s_{i,k}^2 +  \sigma_i s_{i,k} s_{k,i} + \sigma_i s_{k,i} s_{i,k} + \sigma_k s_{k,i}^2}{\sigma_k^2 - \sigma_i^2}.
\end{align}

\subsection{Case 2: $\sigma_i = 0$}

\begin{align}
    d^2\sigma_k|_{\sigma_i = 0} = \frac{1}{\sigma_k} \sum_{i=r+1}^{\max(m,n)} \left( s_{i,k}^2 + s_{k,i}^2 \right).
\end{align}

\subsection{Total Second-Order derivative}

    \begin{lemma}
        \begin{align}
           d^2\sigma_k = d^2\sigma_k|_{\sigma_i \neq 0} + d^2\sigma_k|_{\sigma_i = 0}  .
        \end{align}
    \end{lemma}

\section{Hessian}

Using the property:
\begin{align}
   \operatorname{vec}(AXB) = (B^T \otimes A)  \operatorname{vec}(X).
\end{align}

Hence:
\begin{align}
    s_{i,k} &= u_i^\top dA v_k \\
    &=\operatorname{vec}(dA)^\top (v_k \otimes u_i)
\end{align}
and:
\begin{align}
    s_{k,i} &= u_k^\top dA v_i \\
    &= \operatorname{vec}(dA)^\top (v_i \otimes u_k).
\end{align}

\begin{theorem}
    We have:
\begin{align}
    \frac{\partial^2 \sigma_k}{d A^2} &= \frac{\partial}{\partial \operatorname{vec}(A)} \operatorname{vec}\left(\frac{\partial \sigma_k}{\partial A}\right) \\
    &=\sum_{i=1, i\neq k}^{r}  \frac{\sigma_k}{\sigma_k^2 - \sigma_i^2} \left[ (v_k v_k^\top) \otimes (u_i u_i^\top) + (v_i v_i^\top) \otimes (u_k u_k^\top) \right] \\
    &\qquad + \sum_{i=1, i\neq k}^{r}  \frac{\sigma_i}{\sigma_k^2 - \sigma_i^2} \left[ (v_k v_i^\top) \otimes (u_i u_k^\top) + (v_i v_k^\top) \otimes (u_k u_i^\top) \right] \\
    &\qquad + \frac{1}{\sigma_k} \sum_{i=r+1}^{i\leq m} (v_k v_k^\top) \otimes (u_i u_i^\top) \\
    &\qquad + \frac{1}{\sigma_k} \sum_{i=r+1}^{i\leq n}  (v_i v_i^\top) \otimes (u_k u_k^\top) \\
    &=\sum_{i=1, i\neq k}^{r}  \frac{\sigma_k}{\sigma_k^2 - \sigma_i^2} \left[  \left(v_k \otimes u_i\right) \left(v_k \otimes u_i\right)^\top   + \left(v_i \otimes u_k\right) \left(v_i \otimes u_k\right)^\top \right] \\
    &\qquad + \sum_{i=1, i\neq k}^{r}  \frac{\sigma_i}{\sigma_k^2 - \sigma_i^2} \left[  (v_k \otimes u_i) (v_i \otimes u_k)^\top  +  (v_i \otimes u_k)(v_k \otimes u_i)^\top \right] \\
    &\qquad + \frac{1}{\sigma_k} \sum_{i=r+1}^{i\leq m} (v_k \otimes u_i) (v_k \otimes u_i)^\top \\
    &\qquad + \frac{1}{\sigma_k} \sum_{i=r+1}^{i\leq n}  (v_i \otimes u_k)(v_i \otimes u_k)^\top \\
    &= \underbrace{\sum_{i \neq k, i \leq m} \frac{\sigma_k}{\sigma_k^2 - \sigma_i^2}\left(v_k \otimes u_i\right)\left(v_k \otimes u_i\right)^\top}_{\text{left}} +\\
    &\qquad \underbrace{\sum_{j \neq k, j \leq n} \frac{\sigma_k}{\sigma_k^2 - \sigma_j^2} \left(v_j \otimes u_k\right)\left(v_j \otimes u_k\right)^\top}_{\text{right}} + \\
    &\qquad \underbrace{\sum_{l \neq k, l \leq r} \frac{\sigma_l}{\sigma_k^2 - \sigma_l^2}\left[ \left(v_k \otimes u_l\right)\left(v_l \otimes u_k\right)^\top + \left(v_l \otimes u_k\right)\left(v_k \otimes u_l\right)^\top \right]}_{\text{left-right interaction}}
\end{align}
\label{theo:hessian_sigma_k}
\end{theorem}

\boxed{
\begin{aligned}
H &= \sum_{i \neq k, i \leq m} \frac{\sigma_k}{\sigma_k^2 - \sigma_i^2}\left(v_k \otimes u_i\right)\left(v_k \otimes u_i\right)^\top + \\
&\quad \sum_{j \neq k, j \leq n} \frac{\sigma_k}{\sigma_k^2 - \sigma_j^2} \left(v_j \otimes u_k\right)\left(v_j \otimes u_k\right)^\top + \\
&\quad \sum_{l \neq k, l \leq r} \frac{\sigma_l}{\sigma_k^2 - \sigma_l^2}\left[ \left(v_k \otimes u_l\right)\left(v_l \otimes u_k\right)^\top + \left(v_l \otimes u_k\right)\left(v_k \otimes u_l\right)^\top \right].
\end{aligned}
}

\begin{align}
H &= \sum_{j=2}^{r} \frac{1}{\sigma_1^2 - \sigma_j^2} \left[ \sigma_1 \left( (u_j \otimes v_1)(u_j \otimes v_1)^T + (u_1 \otimes v_j)(u_1 \otimes v_j)^T \right) \right]+ \\
&\qquad \sum_{j=2}^{r} \frac{1}{\sigma_1^2 - \sigma_j^2}\left[\sigma_j \left( (u_j \otimes v_1)(u_1 \otimes v_j)^T + (u_1 \otimes v_j)(u_j \otimes v_1)^T \right) \right] + \\
&\qquad \sum_{j=r+1}^{m} \frac{1}{\sigma_1} \left( u_j \otimes v_1 \right) \left( u_j \otimes v_1 \right)^T + \sum_{j=r+1}^{n} \frac{1}{\sigma_1} \left( u_1 \otimes v_j \right) \left( u_1 \otimes v_j \right)^T    
\end{align}
